# Supplementary material for: Towards Visual Semantics
Source: arXiv:2104.12379 source file (2021-09-14)
Supplement: Supplementary file 1 [file supplementary.tex]

\relax
%File: formatting-instructions-latex-2021.tex
%release 2021.1
\documentclass[letterpaper]{article} % DO NOT CHANGE THIS
\usepackage{aaai21}  % DO NOT CHANGE THIS
\usepackage{times}  % DO NOT CHANGE THIS
\usepackage{helvet} % DO NOT CHANGE THIS
\usepackage{courier}  % DO NOT CHANGE THIS
\usepackage[hyphens]{url}  % DO NOT CHANGE THIS
\usepackage{graphicx} % DO NOT CHANGE THIS
\urlstyle{rm} % DO NOT CHANGE THIS
  % DO NOT CHANGE THIS
\usepackage{natbib}  % DO NOT CHANGE THIS AND DO NOT ADD ANY OPTIONS TO IT
\usepackage{caption} % DO NOT CHANGE THIS AND DO NOT ADD ANY OPTIONS TO IT
\frenchspacing  % DO NOT CHANGE THIS
\setlength{\pdfpagewidth}{8.5in}  % DO NOT CHANGE THIS
\setlength{\pdfpageheight}{11in}  % DO NOT CHANGE THIS
%\nocopyright
%PDF Info Is REQUIRED.
% For /Author, add all authors within the parentheses, separated by commas. No accents or commands.
% For /Title, add Title in Mixed Case. No accents or commands. Retain the parentheses.
\pdfinfo{
/Title (AAAI Press Formatting Instructions for Authors Using LaTeX -- A Guide)
/Author (AAAI Press Staff, Pater Patel Schneider, Sunil Issar, J. Scott Penberthy, George Ferguson, Hans Guesgen, Francisco Cruz, Marc Pujol-Gonzalez)
/TemplateVersion (2021.1)
} %Leave this

\setcounter{secnumdepth}{0} %May be changed to 1 or 2 if section numbers are desired.

% The file aaai21.sty is the style file for AAAI Press
% proceedings, working notes, and technical reports.
%

\input{pm_macros}
% Use the postscript times font!
\usepackage{import}
\usepackage{soul}
\usepackage[utf8]{inputenc}
\usepackage{amsmath}
\usepackage{amssymb}
\usepackage{amsthm}
\usepackage{booktabs}
\usepackage{algorithm}
\usepackage[noend]{algpseudocode}
\usepackage{bbm}
\usepackage{calc}
\usepackage{textcomp}
\usepackage{color}
\usepackage{mathtools}

\ifdefined\releaseversion
    \newcommand{\andrea}[1]{}
    \newcommand{\luca}[1]{}
    \newcommand{\fausto}[1]{}
\else
    \newcommand{\andrea}[1]{{\bf \textcolor{blue}{Andrea: #1}}}
    \newcommand{\luca}[1]{{\bf \textcolor{cyan}{Luca: #1}}}
    \newcommand{\fausto}[1]{{\bf \textcolor{red}{Fausto: #1}}}
\fi

\usepackage{standalone}
\usepackage{tikz}
\import{figures/}{tikzcommon}
\import{./}{commondef}

\title{%Memory-based hierarchical visual object learning
A solution to the Semantic Gap problem -- Appendix}

% \author{%
% Fausto Giunchiglia\and
% Luca Erculiani\and
% Andrea Passerini \\
% }
% \affiliations{
% University of Trento, Italy\\
% %$^2$School of Artificial Intelligence, Jilin University, Changchun, China, CN \\
% %{\it name.surname}@unitn.it
% }

\begin{document}

\maketitle

\import{sections/}{appendixAAAI}

\bibliography{ref}
\end{document}
